# Supplementary material for: SciXGen: A Scientific Paper Dataset for Context-Aware Text Generation
Source: arXiv:2110.10774 source file (2021-10-20)
Supplement: Supplementary file 1 [file appendix.tex]

\appendix
\section{Appendix}

\subsection{Dataset Construction}
\subsubsection{LaTeX parser}
Our LaTeX parser extracts information from the XML formatted output.
The XML document contains 109 distinct types of tags which are used to identify different contents (e.g., <float>, <table>, <tabular>, <section>). Our objective is to increase the amount of information retained in the LaTeX source data. Therefore, we precisely design the method that is used to process each tag. Among these tags, <Error> indicates LaTeXML encounters an unknown symbol during the parsing process. In practice, we retain the text that is contained inside. 
Additionally, the objects in the paper are manually categorized into 7 classes (i.e. table, figure, algorithm, theorem, verbatim and text) according to the tags.

\subsubsection{Auxiliary LaTeX parser}
Our auxiliary LaTeX parser is fully self-contained.
We use it to parse a paper when LaTeXML fails.
Different from the parser above that parse the data from an intermediate format (i.e. XML), this auxiliary LaTeX parser directly parse data from the source.
To deal with different objects in the paper (e.g., tables, figures), we extract all blocks that start with the symbol ``$\backslash$begin'' with the object types followed, to the symbol ``$\backslash$end''.
After calculation, there are over 6000 object types over the source codes, which makes us difficult to deal with each of them.
Therefore, we employ a neural network to classify these object types into 7 classes (i.e. table, figure, algorithm, theorem, verbatim and text) and an additional class (i.e. other) for the types such as ``minipage".
To train this model, we manually annotate 1000 samples from the LaTeX source codes. 
As the input to the model, we concatenate the object type name and the content text into a sequence for classification.
Thus, we predict the object class for each block and process them with a well-design method for each object class (e.g., extracting tabular data from table, locating image paths in the figure content). 
To our surprise, our auxiliary LaTeX parser can retain more objects, since this parser is directly run on the source code instead of an intermediate file (i.e. XML). LaTeXML may lose information when parsing the source codes into XML file.
Thus, if the objects in the main LaTeX parser are missing, we use this auxiliary LaTeX parser instead.
The example of our auxiliary LaTeX parser can be found in \url{paperparser.com/latexparser/}. 
It should be noted that we have made many efforts to create a robust LaTeX parser from scratch, such as: 1) finding the entry of the source code, 2) removing the comments, 3) replacing user-defined commands , 4) extracting body text and so on.
However, as our auxiliary LaTeX parser does not rely on any LaTeX library, the accuracy of parsing body text from millions of symbols remains challenging; hence, we only use this parser as an auxiliary.

\subsubsection{Bibliography reference resolution}
Bibliography Reference Resolution requires us to first locate the entities involved in the bibliography entries, such as titles, authors, dates and more. In this work, we use a BERT model in training (original settings as bert-base-uncased). As shown in Table~\ref{tab:ner}, all entities can be predicted near-perfectly, indicating that this model can be appropriately used in our work.

Then, we use the title and author information to match a full-text paper. To be specific, we calculate the edit distance between our title and all the titles from the external database. As our BERT models sometimes make mistakes on locating the titles or the authors, we set a threshold to first filter out most of the candidates. Then, we check the names of the authors to keep the paper that contains the same author. In this step, we design different methods to match the names according to their forms (i.e. abbreviation or full name). Finally, we select the one with the lowest distance as our linked paper or we record -1 if there is no candidate left.
\begin{table}[]
\centering
\begin{tabular}{lcc}
\hline
Entity      & Precision & Recall \\\hline
note        & 99.21     & 99.08  \\
volume     & 98.62     & 99.20  \\
date        & 99.82     & 99.69  \\
title       & 99.41     & 99.48  \\
journal     & 98.34     & 98.29  \\
publisher   & 98.42     & 98.62  \\
tech        & 98.35     & 97.86  \\
institution & 97.43     & 98.06  \\
pages       & 99.78     & 99.27  \\
location    & 98.90     & 99.06  \\
booktitle   & 98.82     & 98.74  \\
editor      & 99.06     & 99.59  \\
author      & 99.82     & 99.89 \\\hline
\end{tabular}
\caption{Accuracy of name entity recognition on bibliography reference resolution.}
\label{tab:ner}
\end{table}

\subsection{Ablation Study}

\subsubsection{Performance of various pre-trained language models}
In the experiment, we use LED-base as the generator for all baselines. 
In this section, we do several ablation studies using different language models. 
We conduct the experiment on context-aware description generation for tables and employ {$x$+$C$(20)}) as input.
We test on BART-base~\cite{lewis2019bart}, BART-large, T5-base~\cite{2020t5} and T5-large. 
As shown in Table~\ref{tab:lm}, the language model achieves superior performance using the same model architecture but more parameters(*-base and *-large).
However, the text generation performance varies significantly across different architectures. BART models outperform others in most of the automatic metrics while getting higher perplexity compared with T5.
That might be related to the different corpora that are used during their training.
The inconsistency of perplexity and other automated metrics further points out the drawback of using automatic criteria in these tasks.

\begin{table*}[tb]
\centering
\begin{tabular}{lllll}\hline
Input          & PPL  & BLEU4 & METEOR & MSCORE \\\hline
$x$+$C$(10)+OFiD(10)      & \textbf{17.81} &  \textbf{2.03}  & \textbf{18.43}      & \textbf{0.12}       \\
$x$+$C$(10)+FiD(10)       & 18.30 & 1.88  & 17.88   & 0.12 \\\hline     
\end{tabular}
\caption{Results using OFiD and FiD to retrieve sentences. As previously mentioned, OFiD retains the order between sentences, while the original FiD ignores it.}
\label{tab:fidrag}
\end{table*}

\subsubsection{FiD vs OFiD}
In context-aware description generation, we use OFiD as our retrieval-augmented model. In this section, we also compare OFiD with original FiD, which ignores the order information in the context. We take $x$+$C$(20) as our input. As shown in Table~\ref{tab:fidrag}, OFiD outperforms FiD in automatic scores, that proves the order information is critical when retrieving from the context with sentences in order. 

\subsubsection{Performance in description generation for theorem}
Compared with models with different objects as input, surprisingly, description generation for theorem achieves the lowest perplexity and highest automatic scores. From our observation, we discover that the equations in the target is the reason of low perplexity and high automatic scores, as many symbols are inside the equations. 
We compare the model with the input $x$+$C$(20) and the input $x$+$C$(20)+mask, which masks all the equations in the target.
As shown in Table~\ref{tab:mask}, we can see that the automatic score rapidly drops when the equations are masked in the target. From the results, we claim that the automatic metrics are vulnerable to equations.
Therefore, it is worthwhile to develop new metrics to measure the generated texts which contain equations accurately. We put this into our future work.

\subsubsection{Case study}
We put case studies for context-aware description generation for tables (Table~\ref{tab:table-case}), figures (Table~\ref{tab:figure-case}), algorithms (Table~\ref{tab:algo-case}), theorems (Table~\ref{tab:theorem-case}) and context-aware paragraph generation (Table~\ref{tab:para-case}).
We highlight the plausible phrases that we consider in the generated texts.
From the result in context-aware paragraph generation, we can see that without the help of context, the generated descriptions are full with factual incorrect sentences.
We further visualize the text in the generated paragraph that can be inferred from the abstract ({\color{blue} blue}) and the retrieved passages ({\color{red} red}).

\begin{table*}[t]
\centering
\begin{tabular}{lcccccccc}
\hline
Input      & \#P(M) & \#Mem(GB) & PPL   & BLEU4 & METEOR  & MOVERS \\\hline
Bart-base  & 129    & 6.6       & 14.43 & 2.01   & 17.85   & 0.14   \\
Bart-large & 406    & 16.0      & 14.15 & \textbf{2.43}   & \textbf{20.64}    & \textbf{0.15}   \\
T5-base    & 220    & \ \ 9.6       & \ \ 9.97  & 1.74   & 17.52   & 0.13   \\
T5-large   & 770    & 23.7      & \ \ \textbf{9.11}  & 2.16   & 18.22    & 0.13   \\
LED-base   & 162    & \ *6.8       & 15.82 & 1.86   & 17.67  & 0.12  \\\hline
\end{tabular}
\caption{Automatic results with different pre-trained language models.  We report the parameter numbers and the memory usage for batch size 1 to each model. * means the input token length is limited to 1024.}
\label{tab:lm}
\end{table*}

\begin{table*}[tb]
\centering
\begin{tabular}{lcccc}
\hline
Input      & PPL   & BLEU4 & METEOR  & MOVERS \\\hline
$x$+$C$(20)      & \ \ 7.53  & 3.19  & 19.80    & 0.16   \\
$x$+$C$(20)+mask & 15.18 & 1.54  & 15.79    & 0.15  \\\hline
\end{tabular}
\caption{The results of context-aware description generation for theorem. In $x$+$C$(20)+mask, we mask the equations in the target.}
\label{tab:mask}
\end{table*}

\subsection{Evaluation}
\subsubsection{Automatic Metrics}
In this section, we details the automatic metrics that are used to measure the generation.

\noindent\textbf{PPL} denotes perplexity which is a measurement of how well a probability distribution or probability model predicts a sample.

\noindent\textbf{BLEU}~\cite{papineni2002bleu} is a word-overlap based metrics that measures the precision over target text’s n-grams.

\noindent\textbf{METEOR}~\cite{denkowski2014meteor} works on word alignments. It computes one to one mapping of words in generated and reference texts considering the distance in WordNet~\cite{fellbaum2010wordnet}.

\noindent\textbf{MoverScore}~\cite{zhao2019moverscore} is a neural based metrics that computes the distance between the contextual representation of
the output and reference texts. It compare the output against references based on their semantics rather than surface forms.

\subsubsection{Human Evaluation}
Though our annotators are the experts in computer science, they find difficulty in evaluating theorems and algorithms since these tasks require the researchers a great deal of background knowledge to understand the logical meaning inside. It indicates that context-aware description generation tasks for theorems and algorithms remain challenging. In future work, new approaches and evaluation metrics should be proposed for these tasks.

\subsection{Paper Number in Different Categories}

We list the paper number in all categories in Table~\ref{tab:more}. We can see that our SciXGen contains a large number of papers in computer vision and machine learning (> 40,000).

\begin{table}[]
\centering
\footnotesize
\begin{tabular}{lr|lc|lr}
\hline
Class & \#num & Class & \#num & Class  & \#num \\\hline
cs.LG    & 62681 & cs.NA    & 7467  & cs.MA & 2803  \\
cs.CV    & 42541 & cs.NE    & 6485  & cs.CE      & 2364  \\
cs.IT    & 22795 & cs.IR    & 6043  & cs.FL      & 2359  \\
cs.AI    & 20030 & cs.DM    & 5478  & cs.MM      & 2072  \\
cs.CL    & 19327 & cs.GT    & 5088  & cs.GR      & 2005  \\
cs.DS    & 11949 & cs.CY    & 4715  & cs.ET      & 1473  \\
cs.SY    & 11392 & cs.SE    & 4712  & cs.DL      & 1168  \\
cs.CR    & 10913 & cs.CC    & 4431  & cs.AR      & 1130  \\
cs.SI    & 10431 & cs.SD    & 4314  & cs.SC      & 948   \\
cs.RO    & 10020 & cs.HC    & 4292  & cs.OH      & 541   \\
cs.DC    & 9188  & cs.DB    & 3680  & cs.OS      & 347   \\
cs.NI    & 9182  & cs.CG    & 3500  & cs.GL      & 54    \\
cs.LO    & 7548  & cs.PL    & 3480  &            &      \\\hline
\end{tabular}
\caption{The number of papers for each class in SciXGen.}
\label{tab:more}
\end{table}

\subsection{Task Selection}
In this paper, we choose description generation and paragraph generation as tasks, perform experiments on several baselines to evaluate their performance when given contextual information. In context-aware description generation task, we select tables, figures, algorithms and theorems that frequently occur in the paper. However, we omit equations due to several reasons. 1) Most equations lack labels, making us difficult to locate the description in the body text.
2) Equations are also involved in other objects (e.g., algorithms and theorems), so it is unnecessary to create a single task for the equations. 
However, other research directions with equations, such as simplifying the equations or pursuing better equation representation, are also promising.

In paragraph generation, we choose the paragraph in the ``Introduction'' section as our target because, 1) In general, the paragraph in the ``Introduction'' section is most relevant to the abstract. 2) Cited papers from this section involves more relevant contents to the main contribution of the paper.

\subsection{Retrieval for Figures and Theorems}
In the manuscript, we conduct experiments on the retrievers by comparing the retrieved sentences and human-annotated sentences. When retrieving sentences for figures and theorems, we can see that the performance is even lower than rule-based methods (i.e., using the 11-th to 20-th sentences previous to the target). Based on our observation of retrieved sentences, the retriever for theorem tends to retrieve sentences with equations, regardless of whether they are relevant or not. The retriever for figures tend to retrieve sentences randomly, so we cannot find a pattern in these retrieved sentences.
These observations raise a challenging problem when the language model deals with tokens with other modals, and it could be a future work from this paper.

\subsection{Figure Types Classifier}
This classifier is used to select the figures that contain charts and bars for context-aware description generation. 
We manually annotate 500 chart/bar images and 500 images without a chart/bar (800/100/100 for train/validation/text).
Then we use ResNet~\cite{he2016deep} to train this classifier. 
As a result, we can achieve over 95\% accuracy on the binary classification.

\subsection{More Implementation Details}
We use PyTorch~\cite{paszke2017automatic} and HuggingFace~\cite{wolf2019huggingface} to implement all the models.
For the pre-trained language models, we use the original version in HuggingFace.
We optimize the parameters with the cross-entropy loss function using the AdamW~\cite{loshchilov2018decoupled} optimizer.
The learning rate was initialized at 4e-5 and got a linear schedule with warm-up at the first 10,000 iterations. 
We finetune the models in all tasks for 10 epochs with the same random seed, record the evaluation of each epoch and report the best results.
We use the cross-entropy loss as the objective function during the training.
We run the experiments using 4 Nvidia A100 GPU for a batch size of 4. Each task can be finished within 48 hours.
In the generation, we use Nucleus Sampling~\cite{holtzman2019curious} in the decoder. As the output changes as the random seed changes, we generate the outputs in each task three times with three fixed seeds and report the average scores of automatic metrics.

In context-aware description generation for figures, 
, we use features extracted from ViT~\cite{dosovitskiy2020image} with the size (197, 768). To fit the hidden size in the language model, we add a randomly initialized projection layer to enlarge its feature size into (197, 1024).

In context-aware paragraph generation, from 42,541 papers in computer vision, we first filter out the papers without the ``Introduction'' section.
Since the decoder has the token length limitation of 1024,  we only keep the target which length is within [200,1000]. Finally, we get 39,523 papers in total.
When we use RAG-sequence to retrieve sentences, we set the maximum combination length as 1024 for the concatenation of each input abstract $a$ and each retrieved passages.

\begin{table*}[]
\small
\begin{tabularx}{\textwidth}{|X|}
\hline
\textbf{Description Generation (Table)}\\\hline
    \begin{tabular}{l|ccccc}

        &  Training IoU  &  mAP@IoU=0.5  &  mAP@IoU=0.6  &  mAP@IoU=0.7 \\\hline
     SSD  &  0.5  &  76.3  &  71.0  &  60.4 \\
     SSD  &  0.7  &  68.4  &  61.9  &  50.8 \\
     SSD w / FPN  &  0.5  &  77.4  &  72.1  &  61.6 \\
     BPN w / o CAR  &  0.5  &  78.1  &  72.7  &  63.4 \\
     BPN w / AR  &  0.5  &  80.0  &  74.2  &  63.6 \\
     BPN w / AR  &  0.7  &  78.1  &  73.7  &  63.1 \\
     BPN  &  (0.5, 0.5, 0.7)  &  80.0  &  75.1  &  65.4 \\
     BPN  &  (0.5, 0.6, 0.7)  &  80.3  &  75.5  &  66.1  \\
    \end{tabular}
\\\hline
\textbf{Gold}
\\\hline
We list the results in Table . Firstly, a vanilla SSD model is trained with 0.7 IoU threshold. This model(Row 2) performs much worse than the baseline(Row 1) trained with 0.5 IoU threshold in all three quality levels, which validates the fact that insufficient positive training samples cause overfitting problem. Secondly, we keep only one CAR block of BPN(dabbed as BPN w / AR), and train this model with 0.5 IoU threshold. The results show the detection results improves significantly compared with BPN w / o CAR in low and mid quality scenarios, but not obvious in high quality case(63.6\% vs 63.4\% ). 
\\\hline
$x$
\\\hline
 In Table we also report the experimental results of the BPN-based model. We observe a consistent drop in accuracy from our models with our AR setting to the same setting of $ (0.5,0.5,0.6) $.
\\\hline
$C$(20)
\\\hline
As shown in Table, we set the level of cascaded up to 4. The higher the cascaded level, the higher the detection accuracy. Therefore, we train with the cascaded level of CAR and vanilla SSD in all possible scenarios.
\\\hline
$x$+$C$(20)
\\\hline
 As shown in Table, as we increase the number of categories in BPN,\hl{there is a drop in mAP from 76.3\% in original SSD to 72.1\%} in BPN w / o CAR, and the drop in mAP from 76.3\% to 70.0\% in our proposed model. So in this experiment we use BPN w / o CAR as baseline model.
\\\hline
$x$+$C$(10)+OFiD(10)
\\\hline
\textbf{10 Retrieved sentences}
\\\hline
\begin{compactitem} 
\item The evaluation metric is mean average precision which is widely used in evaluating object detection.
\item Notably, after refined by CAR we have sufficient positive training samples in high quality levels so that we could conduct gradually increasing training positive IoU thresholds (0.5, 0.6 and 0.7)
\item Bidirectional Feature Pyramid: To validate the effectiveness of the Bidirectional Feature Pyramid, we remove CAR from BPN and compare this model(dabbed as BPN w / o CAR) with vanilla SSD and SSD w / FPN.
\item We use mean average precision on three different IoU thresholds(0.5, 0.6 and 0.7) as our evaluation metric.
\item In Table , we count the positive anchor numbers per image on different IoU thresholds in original SSD, FPN and BPN respectively.
\item In original SSD, anchors are generated manually and only a few anchors matched objects, which is hard to train detectors effectively.
\item Notably, after refined by CAR we have sufficient positive training samples in high quality levels so that we could conduct gradually increasing training positive IoU thresholds (0.5, 0.6 and 0.7).
\item Bidirectional Feature Pyramid: To validate the effectiveness of the Bidirectional Feature Pyramid, we remove CAR from BPN and compare this model(dabbed as BPN w / o CAR) with vanilla SSD and SSD w / FPN.
\item Bidirectional Feature Pyramid is built based on vanilla SSD and all three models are fine-tuned with IoU threshold as 0.5
\item In Table, SSD w / FPN outperforms vanilla SSD because deep semantic features boost feature representations. 
\end{compactitem} 

\\\hline
To validate the effectiveness of the cascaded level we conduct experiments on the BPN-PIRP-v5 (bPN w / SSD) and BPN w / o CAR (bPN w/ R) as shown in Table. \hl{First, BPN w / o CAR improves the performance in both training IoU thresholds and validation IoU thresholds, but in general 2-4\% improvement.} Further, we observe that the performance of BPN w / AR improves the performance of SSD w / o CAR in validation IoU thresholds. We conclude that the cascaded levels of CAR are indispensable to boost the quality of anchor performances. The future work should study more challenging levels of CAR to understand the value of high quality anchor data, which will be discussed in the following section.
\\\hline
$x$+$C$($\infty$)
\\\hline
\hl{In Table, we count the improvements of BPN w / o CAR in different IoU thresholds as our training set and test set when the cascaded level of CAR is 0.5, 0.6 and 0.7.} Overall, with no more than three training samples for each layer, CAR can continuously improve our detection results.
\\\hline
\end{tabularx}
\caption{Case study on table description generation. Highlighted texts are the phrases that can be inferred from the table.}
\label{tab:table-case}
\end{table*}

\begin{table*}[]
\small
\begin{tabularx}{\textwidth}{|X|}
\hline
\textbf{Description Generation (Figure)}\\\hline
\includegraphics[scale=0.15]{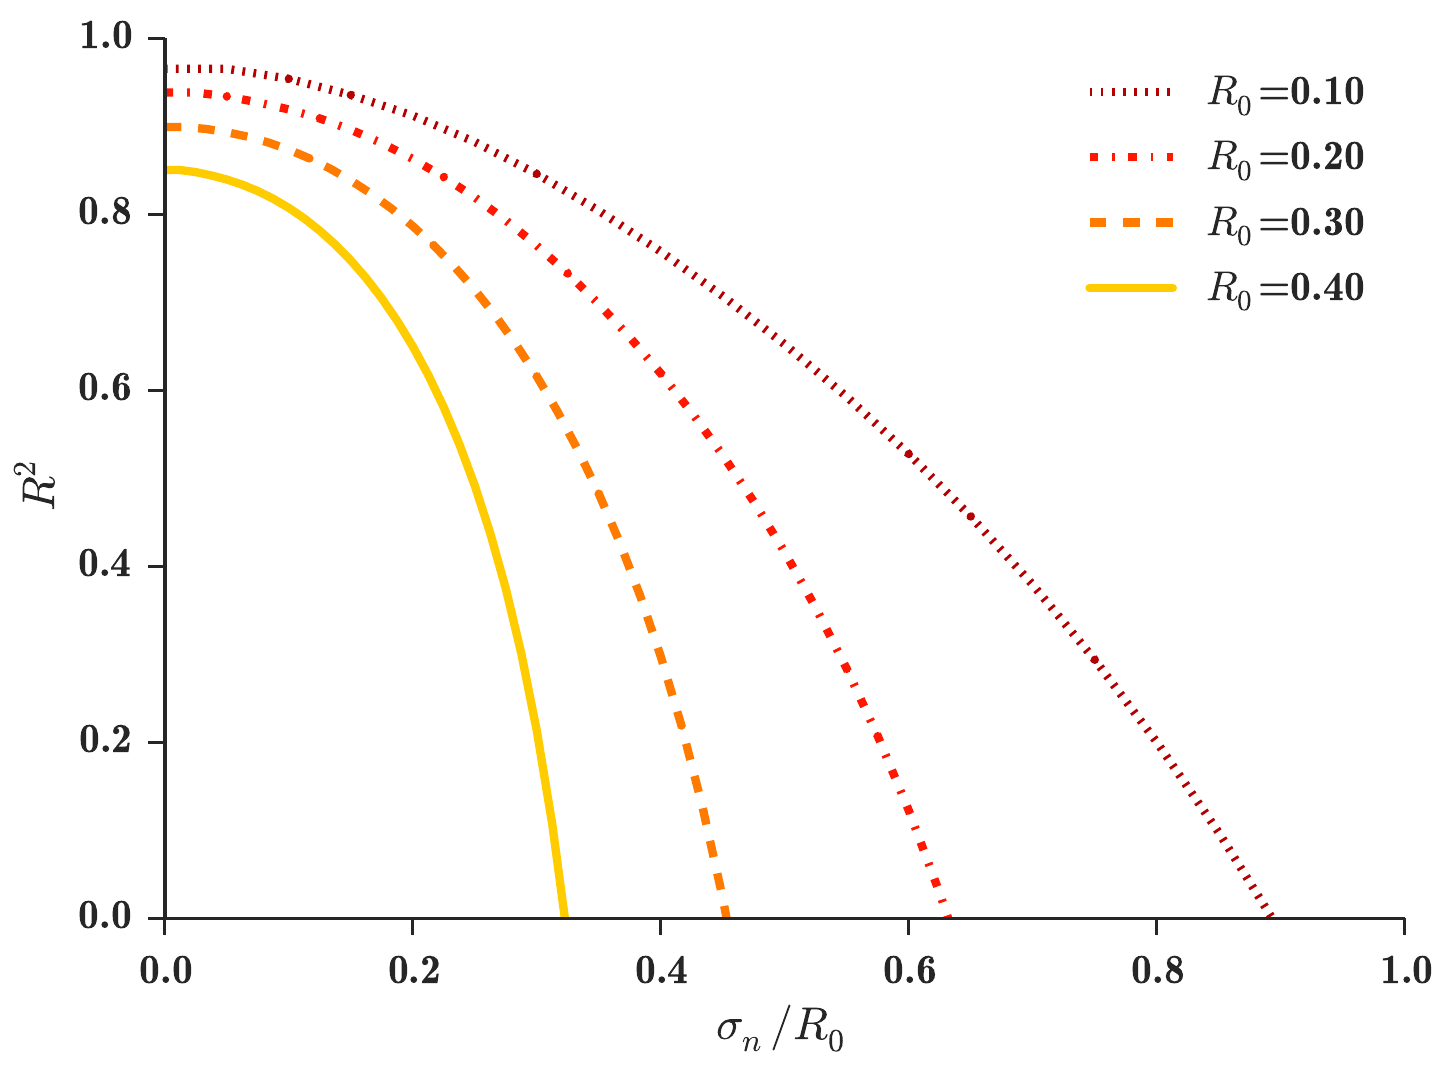}
\\\hline
\textbf{Gold}
\\\hline
We note, moreover, that in Figure we have chosen $ \sigma_{q}=0 $ (i.e. all products have equal $ R_{0} $ ), which we, as we have already established, maximizes predictability in the perfect information case. Introducing heterogeneity in product quality decreases $ R^{2} $ even further.
\\\hline
$x$
\\\hline
As shown in Figure, the fusion strategy significantly improves the translation quality. Interestingly, the improvement is more apparent when using the updated offline algorithm. Instead of tuning the tuning parameter, the updated offline algorithm requires a lower number of models for the documents, which is critical for efficient translation learning.
\\\hline
$C$(20)
\\\hline

Table shows the pose accuracies in human hand and robot arm accuracy. Our ground-truth annotations are better than human hand in some settings. In other words, our annotations make the annotation more accurate in the human hand.
\\\hline
$x$+$C$(20)
\\\hline
Finally, \hl{Figure shows how performance degrades as more knowledge of the product quality is provided.} This is important when one assumes that the main effects of lack of product quality are related to knowledge of high quality.
\\\hline
$x$+$C$(10)+OFiD(10)
\textbf{10 Retrieved sentences}
\\\hline
\begin{compactitem} 
    \item We find that content-based features alone perform poorly, consistent with previous work. 
    \item For example, a model with only basic user features achieves close to 0.2, several times the performance of the best content-only model. 
    \item To summarize, performance increases as we consider more features, significantly outperforming previously reported {ex-ante} prediction results , which achieved $ \approx 0.34 $ .
    \item In our model world, we operationalize the quality/appeal of a particular product in terms of its {reproduction number}, defined as the expected number of new nodes infected by any individual node in a cascade, 
    \item In light of previous work showing that Twitter cascades are best, we sample reproduction numbers from a Beta distribution: $ Beta(q,\sigma_{q}) $. 
    \item To cover a wide range of users and reproduction numbers, we simulate cascades for 10,000 different seed users and 800 uniformly spaced values. 
    \item Having specified our model world, we can investigate the variance in cascade sizes (success) given identical initial conditions.
    \item Specifically we evaluate predictive performance in our simulations the same way we evaluated our empirical models.  
    \item values that are most appropriate for modeling the empirical distribution of cascade size on Twitter, the theoretical maximum prediction performance reduces to $ 0.93 $ . 
\end{compactitem} 

\\\hline
This effect is especially significant when $ R_{0} $ is bounded away from 0.2 as the standard deviation of the magnitude of the cascade size increases (see Figure ). \hl{This suggests that in addition to the typical case of estimating the control kernel $ R_{0} $,} the dynamics of cascades propagate according to previously existing knowledge as well as the known base load. In other words, the errors generated by knowledge of aggregate labels do not spread as far as $ R_{0} $. This is to be expected since a huge amount of \hl{empirical data (hence, $ R^{2}=0.3 $ ) has been collected across the population.}
\\\hline
$x$+$C$($\infty$)
\\\hline
Moreover, in our simulation, \hl{we observe that while $ R^{2} $ is bounded away from 1 for perfect ex-ante knowledge of the system,} predicting performance degrades quite rapidly as a result of quite a few scattered fluctuations in $ R^{2} $ (see Figure ). We emphasize again that our prediction score is just a very small fraction of one’s overall prediction performance without a noticeable drop in prediction performance.
\\\hline
\end{tabularx}
\caption{Case study on figure description generation. Highlighted texts are the phrases that can be inferred from the images.}
\label{tab:figure-case}
\end{table*}

\begin{table*}[]
\small
\begin{tabularx}{\textwidth}{|X|}
\hline
\textbf{Description Generation (Algorithm)}\\\hline
$ \mathsf{Interpolate}({\gamma}^{-},{\gamma}^{+}) $ \\
two constraint sequences $ {\gamma}^{-} $ and $ {\gamma}^{+} $ , with $ {\gamma}^{-}\land{\gamma}^{+} $ is contradicting \\ a constraint sequence $ {\Gamma} $ , which is an interpolant for $ {\gamma}^{-} $ and $ {\gamma}^{+} $ \\ an abstract variable assignment $ v $ \\$ v:={\sf SP}_{{\gamma}^{-}}({\emptyset}) $ \\ for each $ x\in\textrm{def}{(v)} $ do \\ \hspace{0.25cm}if $ {\sf SP}_{{\gamma}^{+}}({v_{|\textrm{def}(v)\setminus\{x\}}}) $ is contradicting then \\ \hspace{0.25cm}// $ x $ is not relevant and should not occur in the interpolant \\ \hspace{0.5cm}$ v:=v_{|\textrm{def}(v)\setminus\{x\}} $ \\ \hspace{0.5cm}// construct the interpolating constraint sequence \\ \hspace{0.5cm}$ {\Gamma}:=\langle\rangle $ \\ \hspace{0.5cm}for each $ x\in\textrm{def}{(v)} $ do \\ \hspace{0.5cm}// construct an assume constraint for $ x $ \\ \hspace{0.75cm}${\Gamma}:={\Gamma}\land\langle[x=v(x)]\rangle $ \\ \hspace{0.75cm}return $ {\Gamma} $ \\

\\\hline
\textbf{Gold}
\\\hline
Algorithm $\mathsf{Interpolate}$ returns an interpolant for two constraint sequences $ {\gamma}^{-} $ and $ {\gamma}^{+} $ . The algorithm starts with computing the strongest post-condition for $ {\gamma}^{-} $ and assigns the result to the abstract variable assignment $ v $ , which then may contain up to $ m $ variables. Per definition, the strongest post-condition for $ {\gamma}^{+} $ of variable assignment $ v $ is contradicting. Next we try to eliminate each variable from $ v $ , by testing if removing it from $ v $ makes the strongest post-condition for $ {\gamma}^{+} $ of $ v $ contradicting (each such test takes $ n $ $ \mathsf{SP} $ steps). If it is contradicting, the variable can be removed. If not, the variable is necessary to prove the contradiction of the two constraint sequences, and thus, should occur in the interpolant. Note that this keeps only variables in $ v $ that occur in $ {\gamma}^{+} $ as well. The rest of the algorithm constructs a constraint sequence from the variable assignment, in order to return an interpolating constraint sequence, which fulfills the three requirements of an interpolant.
\\\hline
$x$
\\\hline
 \hl{$ \mathsf{Interpolate} $ (Algorithm ) construct the interpolant $ {\Gamma} $ for $ \gamma^{-} $ and $ {\gamma}^{+} $ in $ \mathsf{Inpolate} $ and return a constraint sequence $ {\Gamma} $ which is a contradicting constraint sequence in $ {\Gamma} $.}
\\\hline
$C$(20)
\\\hline
 By construction, there exists a sequence of variables $ {\gamma}^{-} $ that is abstracted and can be invoked to construct a constraint sequence $ {\Gamma} $, using Algorithm. If $ {\gamma}^{-} $ is a subset of $ {\gamma}^{-} $, then the union of $ {\gamma}^{-}\land{\gamma}^{+} $ and $ {\gamma}^{+} $ is contradicting.
\\\hline
$x$+$C$(20)
\\\hline
 \hl{We solve the linear regression problem by selecting two constraint sequences $ {\gamma} $ and $ {\gamma}^{+} $, which are strongly contradicting (Algorithm ).} Let $ {\gamma}_{i} $ and $ {\gamma_{j}} $ be two constraint sequences for $ {\gamma}^{-} $ and $ {\gamma}^{+} $ and $ \gamma_{j} $, respectively. Let $ \gamma $ be a constraint sequence that is bound by $ {\gamma}_{i} $.
\\\hline
$x$+$C$(10)+OFiD(10)
\textbf{10 Retrieved sentences}
\\\hline
\begin{compactitem} 
    \item for each variable $ x\in\textrm{def}(v)\cup\textrm{def}(v^{\prime}) $ we have $ (v\land v^{\prime})(x)=\left\{\begin{array}[]{ll}v(x)&\textrm{if }x\in\textrm{def}(v)\textrm{and }x\not\in\textrm{def}(v^{\prime})\\ v^{\prime}(x)&\textrm{if }x\not\in\textrm{def}(v)\textrm{and }x\in\textrm{def\% }(v^{\prime})\\ v(x)&\textrm{if }v(x)=v^{\prime}(x)\\ \bot&\textrm{if }\top\not=v(x)\not=v^{\prime}(x)\not=\top\\ \top&\textrm{otherwise }(v(x)=\top\textrm{or }v^{\prime}(x)=\top)\end{array}\right.$ 
    \item Furthermore we define {contradiction} for an abstract variable assignment $ v $ : $ v $ is contradicting if there is a variable $ x\in\textrm{def}(v) $ such that $ v(x)=\bot $ (which implies $ [\![v]\!]=\emptyset $ ).
    \item Formally, given an abstract variable assignment $ v $ and an assignment operation $ s:=exp $ , we have $ {\sf SP}_{s:=exp}({v})=v_{|{X\setminus\{s\}}}\land v_{s:=exp}$
    \item The {semantics of a program path} $ \sigma=\langle(\mathit{op}_{1},\mathit{l}_{1}),...,(\mathit{op}_{n},\mathit{l} _{n})\rangle $ is defined as the successive application of the strongest post-operator to each operation of the corresponding constraint sequence.
    \item The set of concrete program states that result from running $ \sigma $ is represented by the pair $ (l_{n},{\sf SP}_{{\gamma}_{\sigma}}({v_{0}})) $ , where $ v_{0}=\{\} $ is the initial abstract variable assignment that does not map any variable to a value. 
    \item Every path $ \sigma=\langle(\mathit{op}_{1},\mathit{l}_{1}),...,(\mathit{op}_{n},\mathit{l}_{n})\rangle $ defines a {constraint sequence} $ {\gamma}_{\sigma}=\langle\mathit{op}_{1},...,\mathit{op}_{n}\rangle $ . 
    \item A concrete state $ (l_{n},cd_{n}) $ is {reachable} from a region $ r $ , denoted by $ (l_{n},cd_{n})\in Reach(r) $ , if there exists a feasible program path $ \sigma=\langle(\mathit{op}_{1},\mathit{l}_{1}),...,(\mathit{op}_{n},\mathit{l} _{n})\rangle $ with $ (l_{0},v_{0})\in r $ and $ cd_{n}\in[\![{\sf SP}_{{\gamma}_{\sigma}}({v_{0}})]\!] $ . 
    \item A program path $ \sigma $ is {feasible} if $ {\sf SP}_{{\gamma}_{\sigma}}({v_{0}}) $ is not contradicting, i.e., $ {\sf SP}_{{\gamma}_{\sigma}}({v_{0}})(x)\not=\bot $ for all variables $ x $ in $ \textrm{def}({\sf SP}_{{\gamma}_{\sigma}}({v_{0}})) $ . 
    \item For a given pair $ (v^{-} $ , $ v^{+}) $ of abstract variable assignments, such that $ v^{-}\land v^{+} $ is contradicting, an interpolant exists. 
    \item The variable assignment $ v^{-}_{|\textrm{def}(v^{+})} $ is an interpolant for the pair $ (v^{-} $ , $ v^{+}) $ 
\end{compactitem} 

\\\hline
\hl{To prove the theorem, we need only consider two instantiations of $ \mathsf{Interpolate}({\gamma}^{-} $ and $ {\gamma}^{+} $ of these instantiations, and define $ {\gamma}^{-}\land{\gamma}^{+} $} to be the sets of real numbers in the formula $ \textrm{SP}_{{\gamma}^{-}}(v_{|\textrm{def}(v)\setminus\{x\}}) $ and $ {\gamma}^{+} $ and $ {\gamma}^{+} $, respectively.
\\\hline
$x$+$C$($\infty$)
\\\hline
The algorithm from Algorithm can be obtained by adding an abstract variable assignment $ v $ to an abstract variable assignment $ {\gamma} $, \hl{such that $ {\gamma}^{-}\land{\gamma}^{+} $ is contradicting. The algorithm finds the exact function $ SP $ that assigns to a $ v $ value that the value in $ {\gamma}^{+} $ is contradicting.} This function takes the maximum possible value of the current value of $ {\gamma} $ and $ {\gamma}^{+} $, where $ {\gamma}^{+} $ and $ {\gamma}^{+} $ are computed iteratively and as high as the value of $ {\gamma} $ is. When constructing $ v $, we consider $ {\gamma}^{+} $ with a value $ {\gamma}^{-} $ and a constraint sequence that presents a contradicting constraint sequence. When the vertex assignment $ v $ has been chosen as the $ \Sigma $, then $ {\gamma}^{+} $ is directly computed.
\\\hline
\end{tabularx}
\caption{Case study on algorithm description generation. Highlighted texts are the phrases that can be inferred from the algorithm.}
\label{tab:algo-case}
\end{table*}

\begin{table*}[]
\small
\begin{tabularx}{\textwidth}{|X|}
\hline
\textbf{Description Generation (Theorem)}\\\hline
Theorem 1 . Let $ A $ and $ B $ be two $ n\times n $ real symmetric matrices such that $ A $ is positive definite and $ B $ is positive semidefinite. Then $ A\succeq B $ if and only if $ \rho(A^{-1}B)\leq 1, $ and $ A\succ B $ if and only if $ \rho(A^{-1}B)<1 $ . 
\\\hline
\textbf{Gold}
\\\hline
By Theorem , it is immediate to conclude that $ \lambda_{\max}(S^{-1}BA^{-1}B^{T})=\rho(S^{-1}BA^{-1}B^{T})<2 $ if and only if $ 2S\succ BA^{-1}B^{T} $ . This fact be used together with Courant-Fisher.
\\\hline
$x$
\\\hline
 Theorem then directly shows that the positive semidefiniteity condition of such a problem cannot be guaranteed for symmetric matrices $ A,B $. \hl{In particular, it needs to be verified that $ \rho(A^{-1}B)<1 $}. In other words, if a symmetric matrix is positive definite, then the other symmetric matrix is also positive semidefinite.
\\\hline
$C$(20)
\\\hline
 Hence, from Lemma we conclude that all the eigenvalues of $ \mathcal{G} $ are real. The next lemma gives the conditions that all eigenvalues of $ {\cal G} $ are real.
\\\hline
$x$+$C$(20)
\\\hline
 It follows directly from Theorem that there is a subspace of $ {\cal G} $ containing a semidefinite $ (A^{-1}B) $ which is equal to the unique $ (B) $ for any initial guess. This completes the proof.
\\\hline
$x$+$C$(10)+OFiD(10)
\textbf{10 Retrieved sentences}
\\\hline
\begin{compactitem} 
\item The notation $ \rho(A) $ stands for the spectral radius of $ A. $ The matrix $ A\in\mathbb{R}^{n\times n} $ is called symmetric positive definite (SPD), if $ A^{T}=A $ and $ x^{T}Ax>0 $ for all nonzero $ x\in\mathbb{R}^{n}. $ Similarly, the matrix $ A $ is called symmetric positive semidefinite (SPSD), if $ A^{T}=A $ and $ x^{T}Ax\geqslant 0 $ for all $ x\in\mathbb{R}^{n}. $ We write $ A\succ 0 $ $ (A\succeq 0), $ if $ A $ is SPD (SPSD). 
\item Theorem 2 . Let $ A\succ 0 $ , $ S\succ 0 $ and $ B $ and $ C $ be full row rank matrices. 
\item The symbol $ x^{*} $ is used for the conjugate transpose of the vector $ x. $ For any square matrix $ A $ with real eigenvalues, the minimum and maximum eigenvalues of $ A $ are indicated by $ \lambda_{\min}(A) $ and $ \lambda_{\max}(A) $ , respectively. 
\item Without loss of generality, we may assume that $ \lambda\neq 0 $ .
\item Proof. Let $ \lambda $ be an arbitrary eigenvalue of $ \mathcal{G}=\mathcal{P}^{-1}\mathcal{R} $ with the corresponding eigenvector $ w=\left(x;y;z\right) $ . 
\item Here, we focus on preconditioned Krylov subspace methods, especially, the preconditiond GMRES method.  
\item The notation $ \rho(A) $ stands for the spectral radius of $ A. $ The matrix $ A\in\mathbb{R}^{n\times n} $ is called 
\item Evidently matrix $ \cal A $ can be regarded as a $ 2\times 2 $ block matrix using the following partitioning strategy $\mathcal{A}=\left({\begin{array}[]{cc|c}A&{B^{T}}&{0}\\ B&0&C^{T}\\ \hline 0&C&0\\ \end{array}}\right)$. 
\item These assumptions guarantee the existence of a unique solution; see for further details. 
\item If $ x=y^{*} $ then $ x\neq 0 $ by Theorem. If $ y^{*} $ is not zero, then $ x\neq 0 $ since $ (Ax+B^{T}y)=Bx+Sy $ is not zero.
\end{compactitem} 

\\\hline
Thus by Theorem it is constant for both $ A $ and $ B $ if and only if $ \rho(A^{-1}B)=1, $ and $ \rho(B^{-1}B)<1 $. Since we have $ \lambda\neq 0 $, it follows that $ \lambda\neq 0 $ and hence $ \lambda<\lambda\mathcal{R}w $.
\\\hline
$x$+$C$($\infty$)
\\\hline
It follows from Theorem and the fact that the first row rows of \hl{$ A^{-1}B^{T} $ correspond to the matrices} that do not have full row rank that can be represented as eigenvalues of $ \mathcal{G} $
\\\hline
\end{tabularx}
\caption{Case study on theorem description generation. Highlighted texts are the phrases that can be inferred from the theorem. The retriever tend to retrieve a sentence that contains equations.}
\label{tab:theorem-case}
\end{table*}

\begin{table*}[]
\small
\begin{tabularx}{\textwidth}{|X|}
\hline
\textbf{Abstract}
\\ \hline
Knowledge Distillation (KD) based methods {\color{blue} adopt the one-way Knowledge Transfer (KT)} scheme in which {\color{blue}training a lower-capacity student network} is guided by a pre-trained high-capacity teacher network. {\color{blue}Recently, Deep Mutual Learning (DML) presented a two-way KT strategy, showing that the student network can be also helpful to improve the teacher network}. In this paper, {\color{blue}we propose Dense Cross-layer Mutual-distillation (DCM), an improved two-way KT method} in which the teacher and student networks are trained collaboratively from scratch. To augment knowledge representation learning, well-designed {\color{blue}auxiliary classifiers} are added to certain hidden layers of both teacher and student networks. {\color{blue}To boost KT performance, we introduce dense bidirectional KD operations between the layers appended with classifiers.} After training, all auxiliary classifiers are discarded, and thus there are no extra parameters introduced to final models. We test our method on a variety of KT tasks, showing its superiorities over related methods. \\ \hline
\textbf{Retrieved passages}\\ \hline
ImageNet {\color{red}classification} with deep convolutional neural networks$\dots$\\
Fully convolutional networks for {\color{red}semantic segmentation}$\dots$\\
$\dots$performance than state-of-the-art models like ResNext. {\color{red}Another problem is that not only the conventional DNN but also the lightweight DNN model requires huge data in learning$\dots$}\\
They use the {\color{red}pre-trained teacher network as the knowledge representation using shared parameters}$\dots$\\
To better learn a small network, the distillation approach starts with a powerful (deep and/or wide) teacher network (or network ensemble), and then {\color{red}trains a smaller student network to mimic the teacher}$\dots$\\
In this paper, we embrace this observation and introduce {\color{red}the Dense Convolutional Network (DenseNet)}$\dots$\\
$\dots$\\
\hline
\textbf{Introduction (Generated paragraph ($a$+RAG(10)*))}\\\hline

Knowledge Distillation (KD) <cite> <cite> has shown remarkable success in solving a number of computer vision tasks such as {\color{red}classification <cite>, segmentation <cite>}, and regression <cite>. {\color{red}While it has been widely used for some practical applications, it is a cumbersome step for most DNN models}. In order to improve DNN models <cite>, {\color{red}the recent KD based works focus on distilling knowledge from a pre-trained teacher network using shared parameters}, where the loss functions learned from a teacher network are shared by the loss functions learned from a shared network; therefore most recent KD methods <cite> {\color{blue}adopt a one-way KD method.} \\
This work is motivated by the fact that there exists a mutual learning (DML) strategy that is well-studied for KD methods. Recent works <cite> aim to achieve this goal by {\color{blue}training a low-capacity student network to} {\color{red}mimic the teacher network}, where the teacher provides a better representation than the training data. DML takes advantage of two sources of dependencies, which is the fact that they are implicitly learnt. {\color{blue}Recently, deep mutual learning (DML) <cite> introduced a two-way KD strategy which shows that the student network and its teacher are mutually beneficial}. It provides an alternative strategy using two different mechanisms. Firstly, it is able to improve the teacher network in both ways, and the student network is naturally encouraged to learn the structure of the teacher network. However, this two-way KD method still has a significant performance gap compared to other two-way methods relying solely on two-way KD methods on classification tasks. \\
In order to build an effective KD manner for DNN, {\color{blue}we propose the Dense Cross Layer Mutual-Distillation (DCM) framework}, which follows one-way KD method. In the Dense Cross Layer Mutual-Distillation (DCM), the teacher network is used to improve the student network, and the difference between the output features and the output of the student network is represented by two consecutive layer activation. Thus, we employ the information loss of the student net to help the teacher networks, in order to learn the structure of the teacher network. In this way, {\color{blue}Dense Cross Layer Mutual-Distillation reduces the inference time caused by the auxiliary classifiers.} \\
We further adopt a different three-step KD strategy, as it consists of a teacher network and a student network. The student networks are jointly trained through joint performance on a variety of tasks, and the teacher networks are further optimized through reinforcement learning (RL). Then, since the auxiliary classifiers are shared among all layers, we are unable to obtain more performance improvement. As shown in Tab. <cite>, we conduct a two-step KD procedure that consists of a $ T $ -layer student network and a $ T $ -layer teacher network
We apply our one-way KD method to a number of popular two-way KD approaches ({\color{red}Dense-Net-Distillation <cite>, Dense-Net <cite>}, Deep Mutual learning <cite>, and Deep Multimodal Learning (DML) under different experimental frameworks. We show that our two-way KD method is able to surpass three popular DML methods on a variety of tasks. \\
To summarize, the contributions of this paper are three-fold: 
 \begin{itemize}
     \item To the best of our knowledge, {\color{blue}we present the first optimized two-way KD method, called Dense Cross Layer Mutual-Distillation (DCM)}. The experiments reveal that by adding extra auxiliary classifiers rather than using multiple auxiliary classifiers by themselves, our method can learn better depth information. 
     \item {\color{blue}We introduce dense bidirectional KD operations between the layers of both teacher and student networks, which can significantly improve their feature representations.} These non-parametric auxiliary classifiers are also useful in promoting the student networks to learn better features, and thus they can help the student network to learn better representations.
 \end{itemize}
\\ \hline
\end{tabularx}
\caption{Case study on paragraph generation. Highlighted texts in {\color{red}red} are the sentences that can be referred to the retrieved passages. Highlighted texts in {\color{blue}blue} are the sentences that can be referred to the retrieved passages.}
\label{tab:para-case}
\end{table*}
